# Supplementary material for: Interplay between alloying and tramp element effects on temper embrittlement in bcc iron: DFT and thermodynamic insights
Source: arXiv:2403.02186 source file (2024-06-12)
Supplement: Supplementary file 1 [file RTE_Supplementary_data_revision.pdf]

# Supplementary data: Interplay between alloying and tramp element effects on temper embrittlement in bcc iron: DFT and thermodynamic insights

Amin Sakic<sup>a,1,\*</sup>, Ronald Schnitzer<sup>b</sup>, David Holec<sup>b</sup>

<sup>a</sup>Department of Materials Science, Montanuniversität Leoben, Franz Josef-Straße 18, 8700, Leoben, Austria

<sup>b</sup>Christian Doppler Laboratory for Knowledge-based Design of Advanced Steels, Department of Materials Science, Montanuniversität Leoben, Franz Josef-Straße 18, 8700, Leoben, Austria

## 1. Grain boundary structures

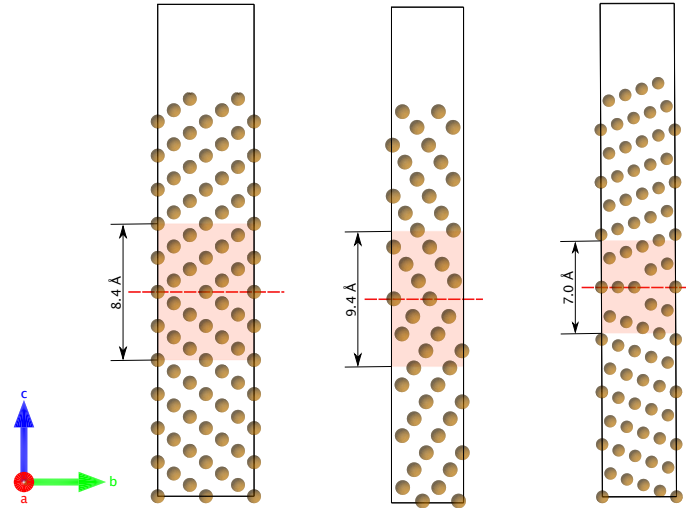

**Figure S1:** The atomic structures of the three GBs studied. The structures of the  $\Sigma 3(1\bar{1}1)[110]$  (left),  $\Sigma 3(1\bar{1}2)[110]$  (middle), and  $\Sigma 9(2\bar{2}1)[110]$  (right). The GB plane is indicated by a red dashed line. The area used to study segregation is highlighted in light gray.

\*Corresponding author

Email addresses: amin.sakic@unileoben.ac.at (Amin Sakic), ronald.schnitzer@unileoben.ac.at (Ronald Schnitzer), david.holec@unileoben.ac.at (David Holec)

<sup>1</sup>amin.sakic@unileoben.ac.at

## 2. Single solute segregation

The single segregation energies for the minimum energy sites are represented and compared to literature values in Table S1. Since we also discuss and compare the impact of P in the main text, its segregation energy is included in here for completeness.

**Table S1:** The segregation energies present at the minimum energy site at each GB studied compared to DFT literature values.

| Species | $E_{seg}$ (eV) – This work |                         |                         | Literature                                                                                                                               |
|---------|----------------------------|-------------------------|-------------------------|------------------------------------------------------------------------------------------------------------------------------------------|
|         | $\Sigma 3(1\bar{1}1)^a$    | $\Sigma 3(1\bar{1}2)^b$ | $\Sigma 9(2\bar{2}1)^c$ |                                                                                                                                          |
| As      | −0.87                      | −0.19                   | −0.98                   |                                                                                                                                          |
| Cr      | −0.12                      | 0.07                    | −0.12                   | −0.03 <sup>a</sup> [1], −0.13 <sup>a</sup> [2], −0.14 <sup>a</sup> [3], −0.18 <sup>a</sup> , −0.07 <sup>b</sup> , −0.21 <sup>c</sup> [4] |
| Mo      | −0.44                      | 0.03                    | −0.40                   | −0.44 <sup>a</sup> [3, 4], −0.61 <sup>a</sup> [5], −0.10 <sup>b</sup> , −0.43 <sup>c</sup> [4]                                           |
| Ni      | −0.39                      | −0.13                   | −0.43                   | −0.31 <sup>a</sup> [1], −0.41 <sup>a</sup> , −0.15 <sup>b</sup> , −0.43 <sup>c</sup> [4]                                                 |
| Sb      | −1.24                      | −0.25                   | −1.15                   | −1.15 <sup>a</sup> [6]                                                                                                                   |
| Sn      | −1.30                      | −0.34                   | −1.33                   | −1.21 <sup>a</sup> [6]                                                                                                                   |
| P       | —                          | —                       | —                       | −1.15 <sup>a</sup> , −0.19 <sup>b</sup> , −1.37 <sup>c</sup> [7], 1.19 <sup>a</sup> [8]                                                  |

For reasons of completeness and clarity, we show in Table S2 the comparison with experimentally or theoretically determined (but not atomistically) segregation energies. The literature values were taken from [9] and compared again with the original papers to exclude possible typing errors.

**Table S2:** The segregation energies present at the minimum energy site at each GB studied compared to experimental literature values.

| Species | $E_{seg}$ (kJ/mol) – This work |                       |                       | Literature                                                                                                                |
|---------|--------------------------------|-----------------------|-----------------------|---------------------------------------------------------------------------------------------------------------------------|
|         | $\Sigma 3(1\bar{1}1)$          | $\Sigma 3(1\bar{1}2)$ | $\Sigma 9(2\bar{2}1)$ |                                                                                                                           |
| As      | −84                            | −18                   | −92                   |                                                                                                                           |
| Cr      | −12                            | 7                     | −12                   | 0 <sup>a</sup> , −16 <sup>b</sup> [10, 9], −3 <sup>c</sup> [11], −8 <sup>d</sup> [10]                                     |
| Mo      | −42                            | 3                     | −39                   | −10 <sup>a</sup> [10, 9], −27 <sup>b</sup> [10, 9], −17 <sup>d</sup> [12], −28 <sup>e</sup> [13]                          |
| Ni      | −38                            | 13                    | −41                   | −4 <sup>a</sup> [10, 9], −20 <sup>b</sup> [10, 9]                                                                         |
| Sb      | −120                           | −24                   | −111                  | −10 <sup>a</sup> [10, 9], −23 <sup>d</sup> [10], −27 <sup>b</sup> [10, 9]                                                 |
| Sn      | −125                           | −33                   | −128                  | −4 <sup>a</sup> [10, 9], −13 <sup>d</sup> [14], −21 <sup>b</sup> [10, 9], −23 <sup>d</sup> [15], <−130> <sup>f</sup> [16] |

<sup>a</sup> Theory, special GB.

<sup>b</sup> Theory, general GB.

<sup>c</sup> Field ion microscopy (FIM), polycrystal.

<sup>d</sup> Auger electron spectroscopy (AES), polycrystal.

<sup>e</sup> Atom probe tomography (APT), 800 °C polycrystal.

<sup>f</sup> Miedema model, polycrystal.

**Table S3:** Summary of the segregation energies in the  $\Sigma 3(1\bar{1}1)[110]$  GB together with site-specific properties of the undecorated GB: distance from the GB plane ( $d_{GB}$ ), site multiplicity ( $m$ ), atomic volume ( $V$ ), and nearest neighbor distance ( $d_{nn}$ ).

| Site | $d_{GB}$ (Å) | $m$ | $V$ (Å <sup>3</sup> ) | $d_{nn}$ (Å) | As    | Cr    | Mo    | Ni    | Sb    | Sn    |
|------|--------------|-----|-----------------------|--------------|-------|-------|-------|-------|-------|-------|
| 1    | 0.0          | 2   | 13.24                 | 2.57         | -0.55 | -0.12 | -0.44 | -0.18 | -1.24 | -1.30 |
| 2    | 1.1          | 4   | 11.29                 | 2.20         | -0.87 | -0.09 | 0.22  | -0.39 | -0.54 | -0.46 |
| 3    | 1.7          | 4   | 12.49                 | 2.39         | -0.44 | -0.04 | -0.18 | -0.09 | -0.59 | -0.67 |
| 4    | 2.6          | 4   | 11.64                 | 2.48         | -0.06 | 0.06  | -0.01 | -0.08 | -0.28 | -0.97 |
| 5    | 3.4          | 4   | 11.38                 | 2.34         | -0.03 | 0.07  | 0.09  | -0.00 | 0.03  | 0.02  |
| 6    | 4.2          | 4   | 11.56                 | 2.45         | -0.10 | 0.03  | -0.01 | -0.00 | -0.21 | -0.25 |
| 7    | 5.1          | 4   | 11.48                 | 2.46         | -0.05 |       |       |       | -0.14 | -0.20 |
| 8    | 5.9          | 4   | 11.43                 | 2.44         | -0.09 |       |       |       | -0.16 | -0.17 |
| 9    | 6.7          | 4   | 11.44                 | 2.45         | -0.09 |       |       |       | -0.19 | -0.20 |
| 10   | 7.5          | 4   | 11.44                 | 2.44         | -0.06 |       |       |       | -0.13 | -0.13 |

**Table S4:** Summary of the segregation energies in the  $\Sigma 3(1\bar{1}2)[110]$  GB together with site-specific properties of the undecorated GB: distance from the GB plane ( $d_{GB}$ ), site multiplicity ( $m$ ), atomic volume ( $V$ ), and nearest neighbor distance ( $d_{nn}$ ).

| Site | $d_{GB}$ (Å) | $m$ | $V$ (Å <sup>3</sup> ) | $d_{nn}$ (Å) | As    | Cr   | Mo   | Ni    | Sb    | Sn    |
|------|--------------|-----|-----------------------|--------------|-------|------|------|-------|-------|-------|
| 1    | 0.0          | 2   | 11.87                 | 2.46         | -0.19 | 0.07 | 0.03 | -0.13 | -0.25 | -0.33 |
| 2    | 1.2          | 4   | 11.81                 | 2.45         | -0.19 | 0.09 | 0.09 | -0.12 | -0.24 | -0.32 |
| 3    | 2.4          | 4   | 11.57                 | 2.45         | -0.19 | 0.12 | 0.10 | -0.13 | -0.24 | -0.32 |
| 4    | 3.5          | 4   | 11.50                 | 2.46         | 0.00  | 0.11 | 0.09 | -0.03 | -0.06 | -0.15 |
| 5    | 4.7          | 4   | 11.43                 | 2.45         | 0.00  | 0.09 | 0.08 | -0.02 | -0.04 | -0.10 |
| 7    | 5.9          | 4   | 11.43                 | 2.46         |       | 0.05 | 0.04 |       |       | -0.09 |
| 8    | 7.0          | 4   | 11.41                 | 2.46         |       | 0.05 | 0.04 |       |       | -0.06 |

**Table S5:** Summary of the segregation energies in the  $\Sigma 9(2\bar{2}1)[110]$  GB together with site-specific properties of the undecorated GB: distance from the GB plane ( $d_{GB}$ ), site multiplicity ( $m$ ), atomic volume ( $V$ ), and nearest neighbor distance ( $d_{nn}$ ).

| Site | $d_{GB}$ (Å) | $m$ | $V$ (Å <sup>3</sup> ) | $d_{nn}$ (Å) | As    | Cr    | Mo    | Ni    | Sb    | Sn    |
|------|--------------|-----|-----------------------|--------------|-------|-------|-------|-------|-------|-------|
| 1    | 0.0          | 1   | 10.86                 | 2.25         | -0.98 | -0.12 | 0.43  | -0.43 | -0.51 | -0.40 |
| 2    | 0.0          | 1   | 12.35                 | 2.44         | -0.29 | 0.05  | -0.16 | -0.12 | -0.89 | -1.17 |
| 3    | 0.0          | 1   | 14.00                 | 2.44         | -0.33 | 0.07  | -0.40 | 0.06  | -1.15 | -1.33 |
| 4    | 1.2          | 2   | 11.90                 | 2.35         | -0.79 | -0.09 | -0.03 | -0.40 | -0.98 | -1.02 |
| 5    | 1.5          | 2   | 12.39                 | 2.46         | -0.21 | -0.06 | -0.30 | -0.12 | -0.61 | -0.77 |
| 6    | 2.1          | 2   | 11.85                 | 2.25         | -0.45 | -0.10 | -0.06 | -0.10 | -0.34 | -0.46 |
| 7    | 2.5          | 2   | 11.69                 | 2.35         | -0.41 | 0.09  | 0.08  | -0.10 | -0.26 | -0.23 |
| 8    | 2.9          | 2   | 12.21                 | 2.46         | -0.32 | 0.01  | -0.08 | -0.11 | -0.53 | -0.59 |
| 9    | 3.5          | 2   | 11.54                 | 2.42         | 0.01  | 0.08  | 0.04  | -0.01 | -0.10 | -0.16 |

## 2.1. Magnetic moment vs. GB distance

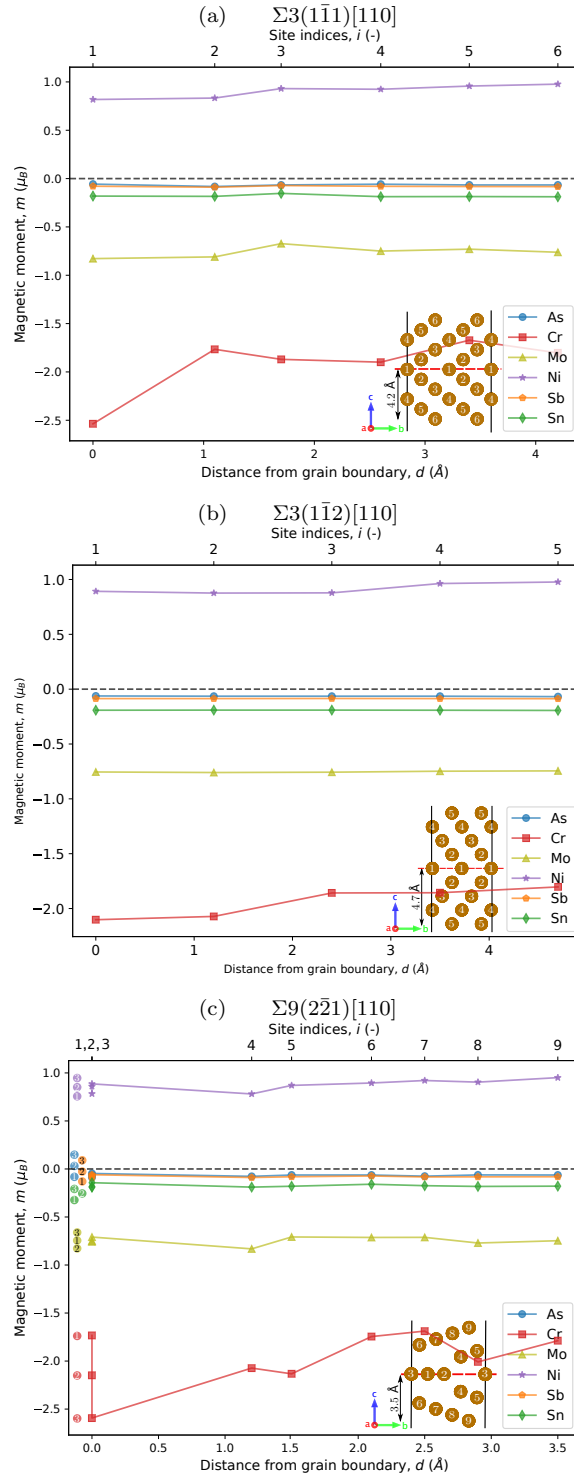

**Figure S2:** Final magnetic moment of the segregants as a function of the GB distance in (a)  $\Sigma 3(1\bar{1}1)$ , (b)  $\Sigma 3(1\bar{1}2)$ , and (c)  $\Sigma 9(2\bar{2}1)$  grain boundaries. The upper x-axis refers to the indexing of sites used in the text.

## 2.2. Impact of elemental segregation on cohesion

**Table S6:** Comparison of the calculated cohesion effects,  $\eta_{RGS}$  (J/m<sup>2</sup>), with previous DFT literature data. A positive sign indicates cohesion enhancement, while a negative sign indicates cohesion reduction.

| Species | $\eta_{RGS}$ (J/m <sup>2</sup> ) - This work |                         |                         | Literature                                                                             |
|---------|----------------------------------------------|-------------------------|-------------------------|----------------------------------------------------------------------------------------|
|         | $\Sigma 3(1\bar{1}1)^a$                      | $\Sigma 3(1\bar{1}2)^b$ | $\Sigma 9(2\bar{2}1)^c$ |                                                                                        |
| As      | -0.74                                        | -1.32                   | -0.61                   |                                                                                        |
| Cr      | 0.08                                         | 0.11                    | 0.21                    | 0.07 <sup>a</sup> , 0.09 <sup>b</sup> , 0.24 <sup>c</sup> [4], 0.09 <sup>a</sup> [3]   |
| Mo      | 0.47                                         | 0.34                    | 0.55                    | 0.33 <sup>a</sup> , 0.40 <sup>b</sup> , 0.40 <sup>c</sup> [4], 0.34 <sup>a</sup> [3]   |
| Ni      | -0.04                                        | -0.17                   | 0.05                    | -0.03 <sup>a</sup> , -0.25 <sup>b</sup> , 0.05 <sup>c</sup> [4], 0.02 <sup>a</sup> [3] |
| Sb      | -0.88                                        | -1.60                   | -0.61                   |                                                                                        |
| Sn      | -0.64                                        | -1.20                   | -0.42                   |                                                                                        |

The impact of segregation on the GB cohesion is represented and compared to literature values in Table S6.

### 3. Co-segregation

#### 3.1. Impact of co-segregation on cohesion

The impact of co-segregated species on the GB cohesion is provided in Table S7.

**Table S7:** Cohesion effect at favored configuration ( $\eta_{X,Y}$  (J/m<sup>2</sup>)). Each row is divided into three sections representing the  $\Sigma 3(1\bar{1}1)$ ,  $\Sigma 3(1\bar{1}2)$ , and  $\Sigma 9(2\bar{2}1)$  GBs. An empty cell signifies that the co-segregation of two species is unfavorable.

|    | As    | Sb    | Sn    | Cr    | Mo    | Ni    |
|----|-------|-------|-------|-------|-------|-------|
| As | -1.56 | -1.67 | -1.45 | -0.72 | -0.45 | -0.82 |
|    | -2.93 | -3.22 | -2.88 | -1.36 | -1.26 | -1.42 |
|    | -1.57 | -1.24 | -1.10 | -0.72 | -0.07 | -0.82 |
| Sb | -1.83 | -1.70 | -1.52 | -0.80 | -0.34 | -0.92 |
|    | -3.22 | -3.81 | -3.80 | -1.63 | -1.47 | -1.65 |
|    | -1.24 | -0.45 | -0.35 | -0.53 | -0.40 | -0.68 |
| Sn | -1.55 | -1.52 | -1.33 | -0.56 | -0.13 | -0.70 |
|    | -2.88 | -3.79 | -3.33 | -1.29 | -1.07 | -1.31 |
|    | -1.10 | -0.51 | -0.37 | -0.40 | -0.21 | -0.55 |
| Cr | -0.72 | -0.80 | -0.56 | 0.21  | 0.63  | 0.04  |
|    | -1.36 | -1.66 | -1.26 | -0.09 | 0.43  | -0.15 |
|    | -0.63 | -0.55 | -0.40 | 0.21  | 0.62  | 0.12  |
| Mo | -0.45 | -0.34 | -0.13 | 0.63  | 1.12  | 0.34  |
|    | -1.28 | -1.47 | -1.07 | 0.43  | 0.43  | 0.06  |
|    | -0.06 | -0.60 | -0.38 | 0.88  | 0.89  | 0.77  |
| Ni | -0.81 | -0.93 | -0.70 | 0.04  | 0.34  | -0.06 |
|    | -1.41 | -1.65 | -1.31 | -0.14 | 0.08  | -0.39 |
|    | -0.63 | -0.69 | -0.55 | 0.18  | 0.76  | 0.06  |

### 3.2. Thermodynamic simulations

For the kinetic simulation, we utilized the diffusion prefactors ( $D_0$ ) and activation energies ( $Q_A$ ) (Table S8) calculated via DFT, as reported in [17]. Finally, using the Arrhenius equation, we computed the diffusion coefficients ( $D$  in  $m^2/s$ ) for each temperature in the kinetic simulation.

**Table S8:** Diffusion prefactors ( $D_0$ ) and activation energies ( $Q_A$ ) in FM bcc-Fe, extracted from [17].

| Solute | $D_0$ ( $m^2/s$ )    | $Q_A$ (eV) |
|--------|----------------------|------------|
| Ni     | $3.6 \times 10^{-5}$ | 2.656      |
| Sb     | $5 \times 10^{-5}$   | 2.424      |
| Sn     | $3.3 \times 10^{-5}$ | 2.355      |

The GB enrichments of Sb and Ni associated with Fig. 5 from the main text are shown in Fig. S3.

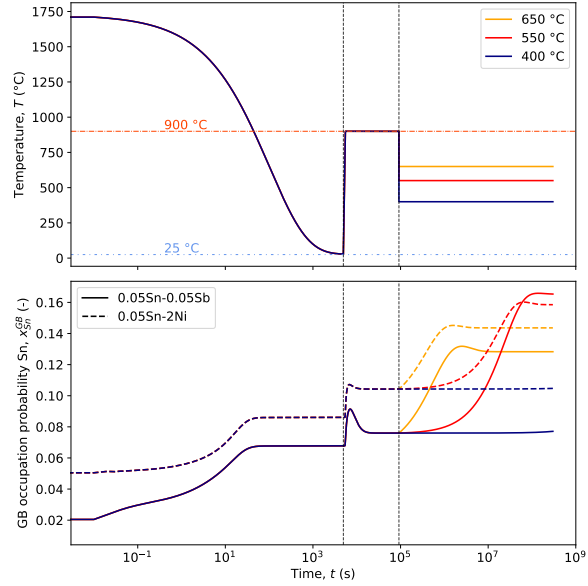

**Figure S3:** GB enrichment of Sb and Ni in the  $\Sigma 3(1\bar{1}1)$  GB for two different alloy compositions in wt.% (bottom panel) and three different isothermal heating temperatures (top panel).

## References

- [1] Z. Xu, S. Tanaka, M. Kohyama, *Journal of Physics: Condensed Matter* **2019**, *31*, 11 115001.
- [2] E. Wachowicz, T. Ossowski, A. Kiejna, *Physical Review B* **2010**, *81*, 9 094104.
- [3] A. S. Kholobina, W. Ecker, R. Pippan, V. I. Razumovskiy, *Computational Materials Science* **2021**, *188* 110215.
- [4] H. L. Mai, X.-Y. Cui, D. Scheiber, L. Romaner, S. P. Ringer, *Acta Materialia* **2022**, *231* 117902.
- [5] Z. Tian, J. Yan, W. Hao, W. Xiao, *Journal of Physics: Condensed Matter* **2010**, *23*, 1 015501.
- [6] M. Yang, J. Zhou, H. Huang, S. Cao, Q. Hu, W. Li, Q. Chen, Y. Qiao, H. Wang, *Journal of Materials Research and Technology* **2023**.
- [7] H. L. Mai, X.-Y. Cui, D. Scheiber, L. Romaner, S. P. Ringer, *Acta Materialia* **2023**, *250* 118850.
- [8] K. Ito, H. Sawada, S. Tanaka, S. Ogata, M. Kohyama, *Modelling and Simulation in Materials Science and Engineering* **2020**, *29*, 1 015001.
- [9] P. Lejček, M. Šob, V. Paidar, *Progress in Materials Science* **2017**, *87* 83.
- [10] P. Lejcek, *Grain boundary segregation in metals*, volume 136, Springer Science & Business Media, **2010**.
- [11] Y. S. Ng, T. Tsong, *Surface Science* **1978**, *78*, 2 419.
- [12] J. Wu, S.-H. Song, L.-Q. Weng, T.-H. Xi, Z.-X. Yuan, *Materials characterization* **2008**, *59*, 3 261.
- [13] N. Maruyama, G. Smith, A. Cerezo, *Materials Science and Engineering: A* **2003**, *353*, 1-2 126.
- [14] M. Seah, C. Lea, *The Philosophical Magazine: A Journal of Theoretical Experimental and Applied Physics* **1975**, *31*, 3 627.
- [15] H. Grabke, *Chemistry and Physics of Fracture* **1987**, 388–415.
- [16] H. A. Murdoch, C. A. Schuh, *Journal of Materials Research* **2013**, *28*, 16 2154.
- [17] C. Versteylen, N. Van Dijk, M. Sluiter, *Physical review B* **2017**, *96*, 9 094105.
